# Supplementary material for: Accurate energies of transition metal atoms, ions, and monoxides using selected configuration interaction and density-based basis-set corrections
Source: arXiv:2109.10271 ancillary file (2021-11-16)
Supplement: Supplementary file 1 [file SI.pdf]

# Supplementary Information for: Accurate energies of transition metal monoxides using selected configuration interaction and density-based basis-set corrections

Yuan Yao,[1,*] Emmanuel Giner,[2,†] Tyler A. Anderson,[1,‡] Julien Toulouse,[2,3,§] and C. J. Umrigar[1,¶]

[1] *Laboratory of Atomic and Solid State Physics, Cornell University, Ithaca, New York 14853, United States*

[2] *Laboratoire de Chimie Théorique, Sorbonne Université and CNRS, F-75005 Paris, France*

[3] *Institut Universitaire de France, F-75005 Paris, France*

## I. BASIS-SET EXTRAPOLATION OF SHCI TOTAL ENERGIES

It has been argued [1–3] that for large basis-set cardinal number, $n$, the correlation energy should converge as

$$E_{\rm corr}^{n{\rm Z}} = E_{\rm corr}^{\rm CBS} + cn^{-3}. \tag{1}$$

However, for small $n$, $E_{\rm corr}$ can deviate considerably from this asymptotic form. For the pseudopotentials and basis sets used in this paper, we find that a much better fit is obtained using

$$E_{\rm corr}^{n{\rm Z}} = E_{\rm corr}^{\rm CBS} + \frac{c}{n^3+d}, \tag{2}$$

which has the same asymptotic behaviour for large $n$. This is demonstrated in Figs. 1, 2, and 3, which show the convergence for the transition metal atoms, ions, and oxides, respectively. The left panels of each figure show the convergence using the usual extrapolation formula of Eq. (1) whereas the right panels show the convergence using the modified extrapolation formula of Eq. (2). Both sets of fits have been weighted by $n^2$. It is apparent that the points fall on the curve far more accurately in the right panels than in the left panels for all 21 systems. In fact, if Eq. (1) is used for extrapolation, then far more accurate extrapolated energies are obtained by fitting only to the largest basis sets, i.e., $n = 4, 5$ rather than fitting to $n = 2, 3, 4, 5$. This is demonstrated in Fig. 4. In every case the extrapolation of Eq. (2) gives a more negative energy than that of Eq. (1) and the latter converge to the former when only the large-$n$ basis sets are used.

Also shown in Fig. 4 is the effect of omitting the $n = 5$ values, i.e., using just $n = 2, 3, 4$ in the extrapolation of Eq. (2) (magenta curve). The largest differences are about 4 mHa, which is not bad considering that the standard extrapolation of Eq. (1) gives errors as big as 6 mHa (blue curve) even when $n = 5$ values are available.

* yy682@cornell.edu
† emmanuel.giner@lct.jussieu.fr
‡ taa65@cornell.edu
§ toulouse@lct.jussieu.fr
¶ cyrusumrigar@cornell.edu

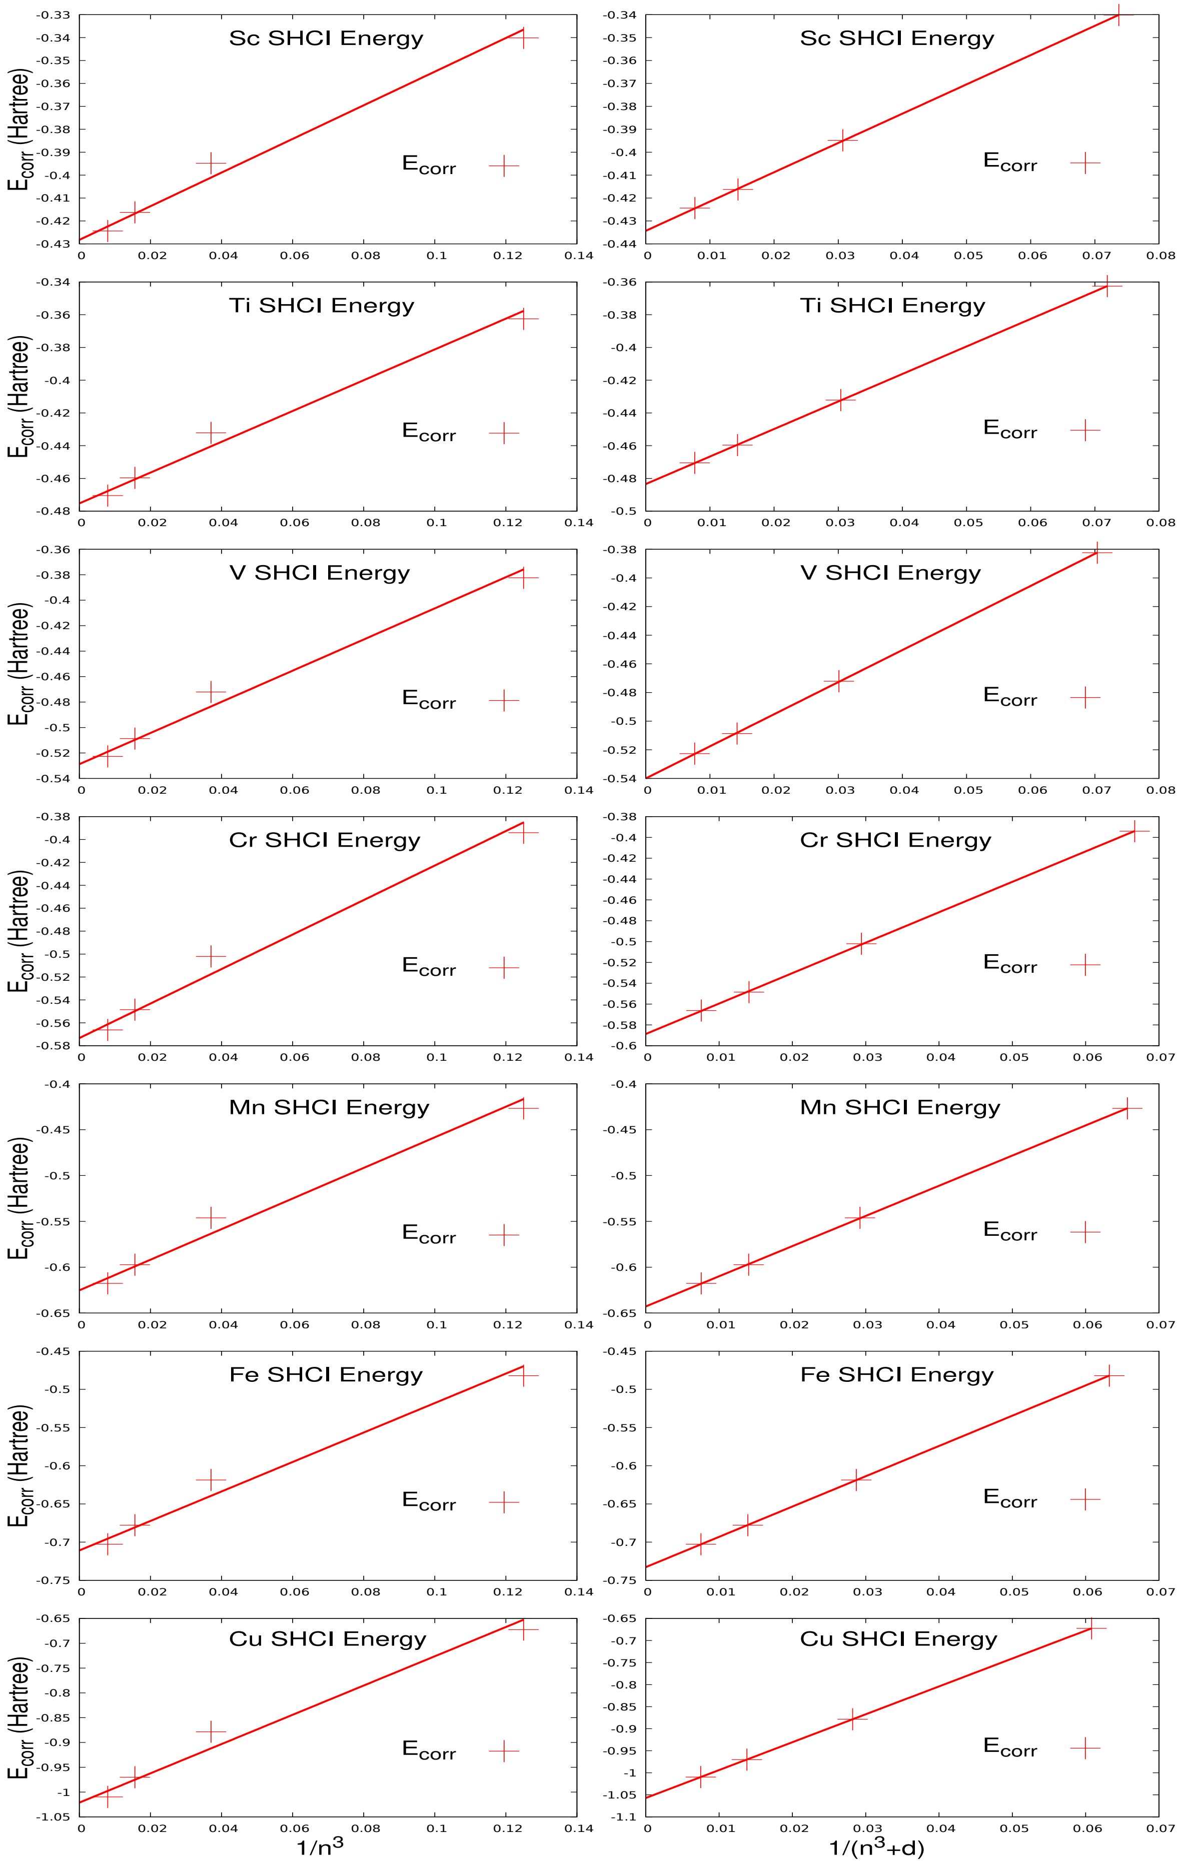


FIG. 1. Demonstration that $c/(n^3 + d)$ gives much better extrapolation fit than $c/n^3$ for transition metal atoms.

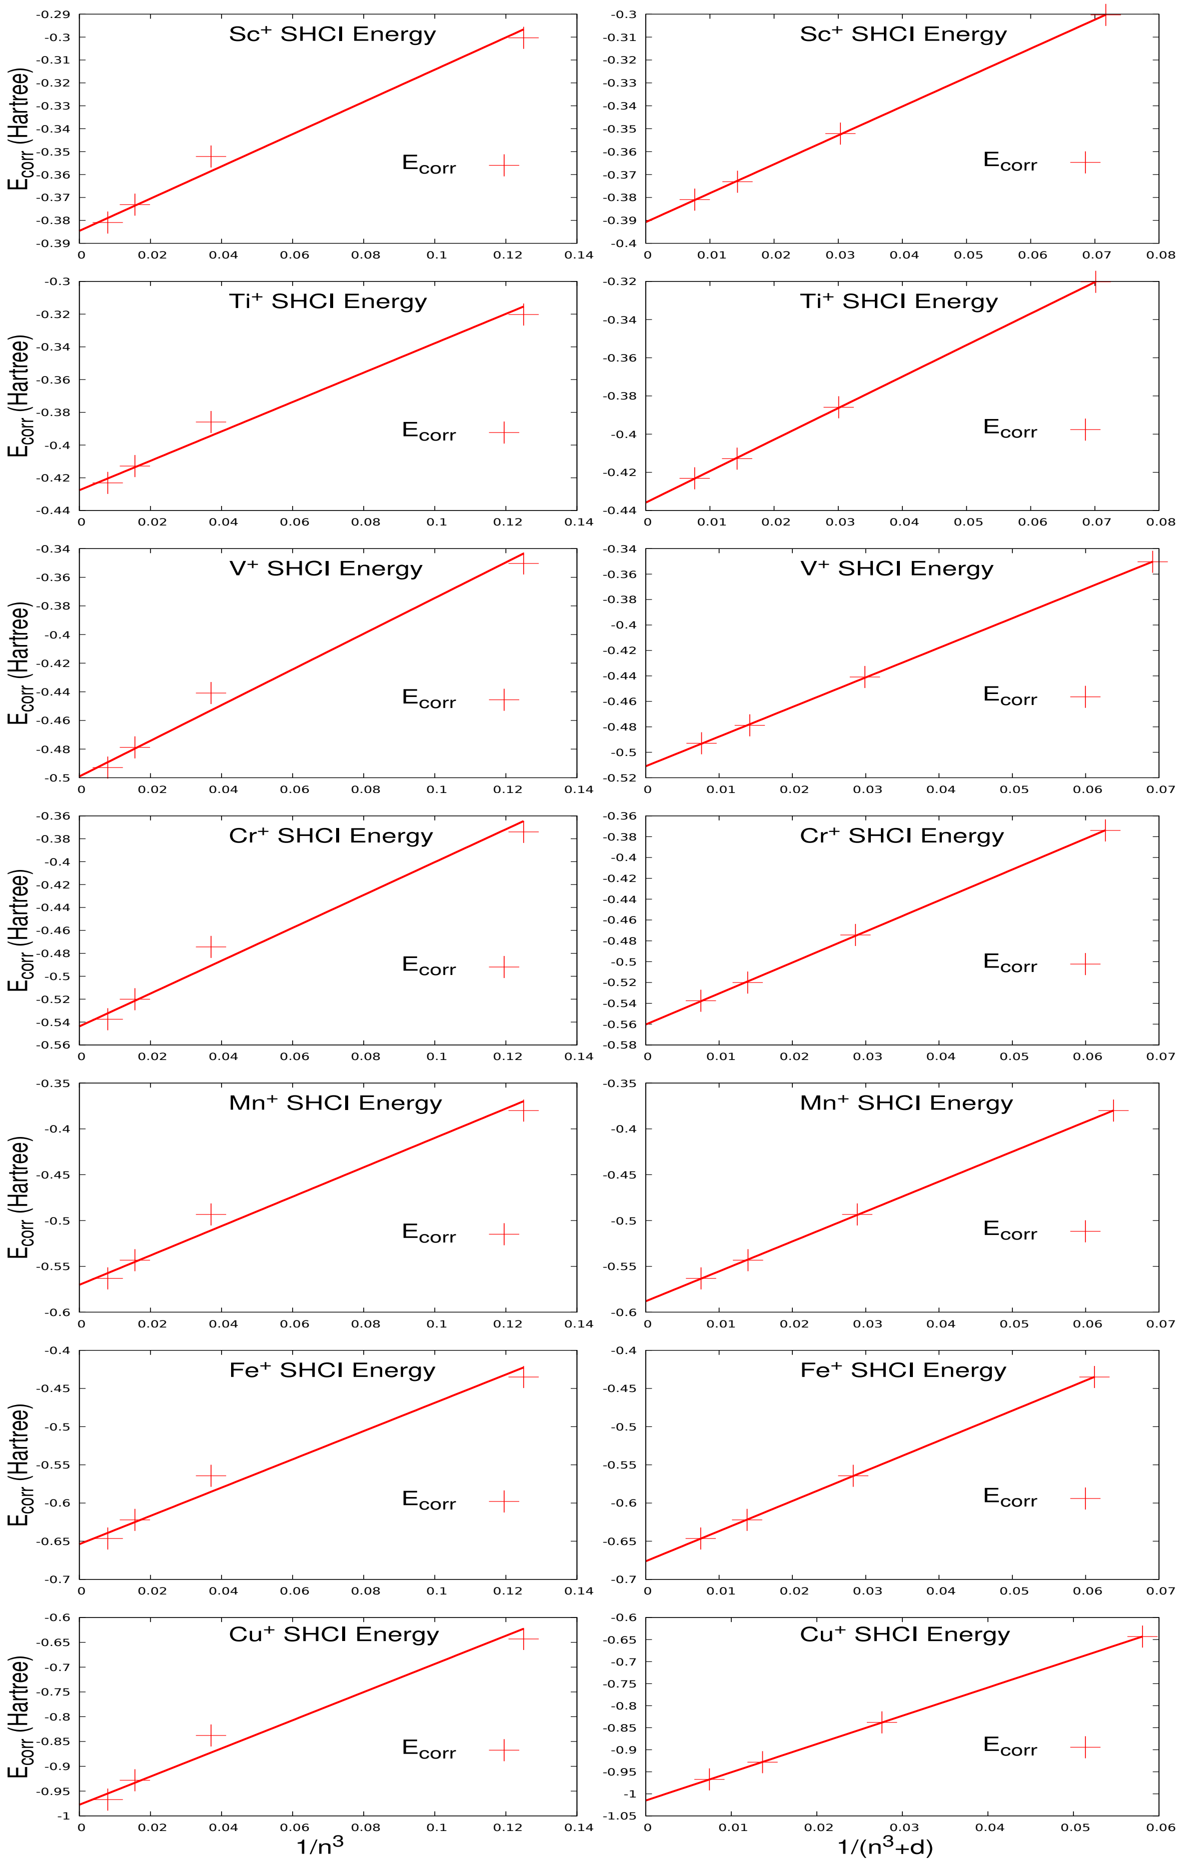


FIG. 2. Demonstration that $c/(n^3+d)$ gives much better extrapolation fit than $c/n^3$ for transition metal ions.

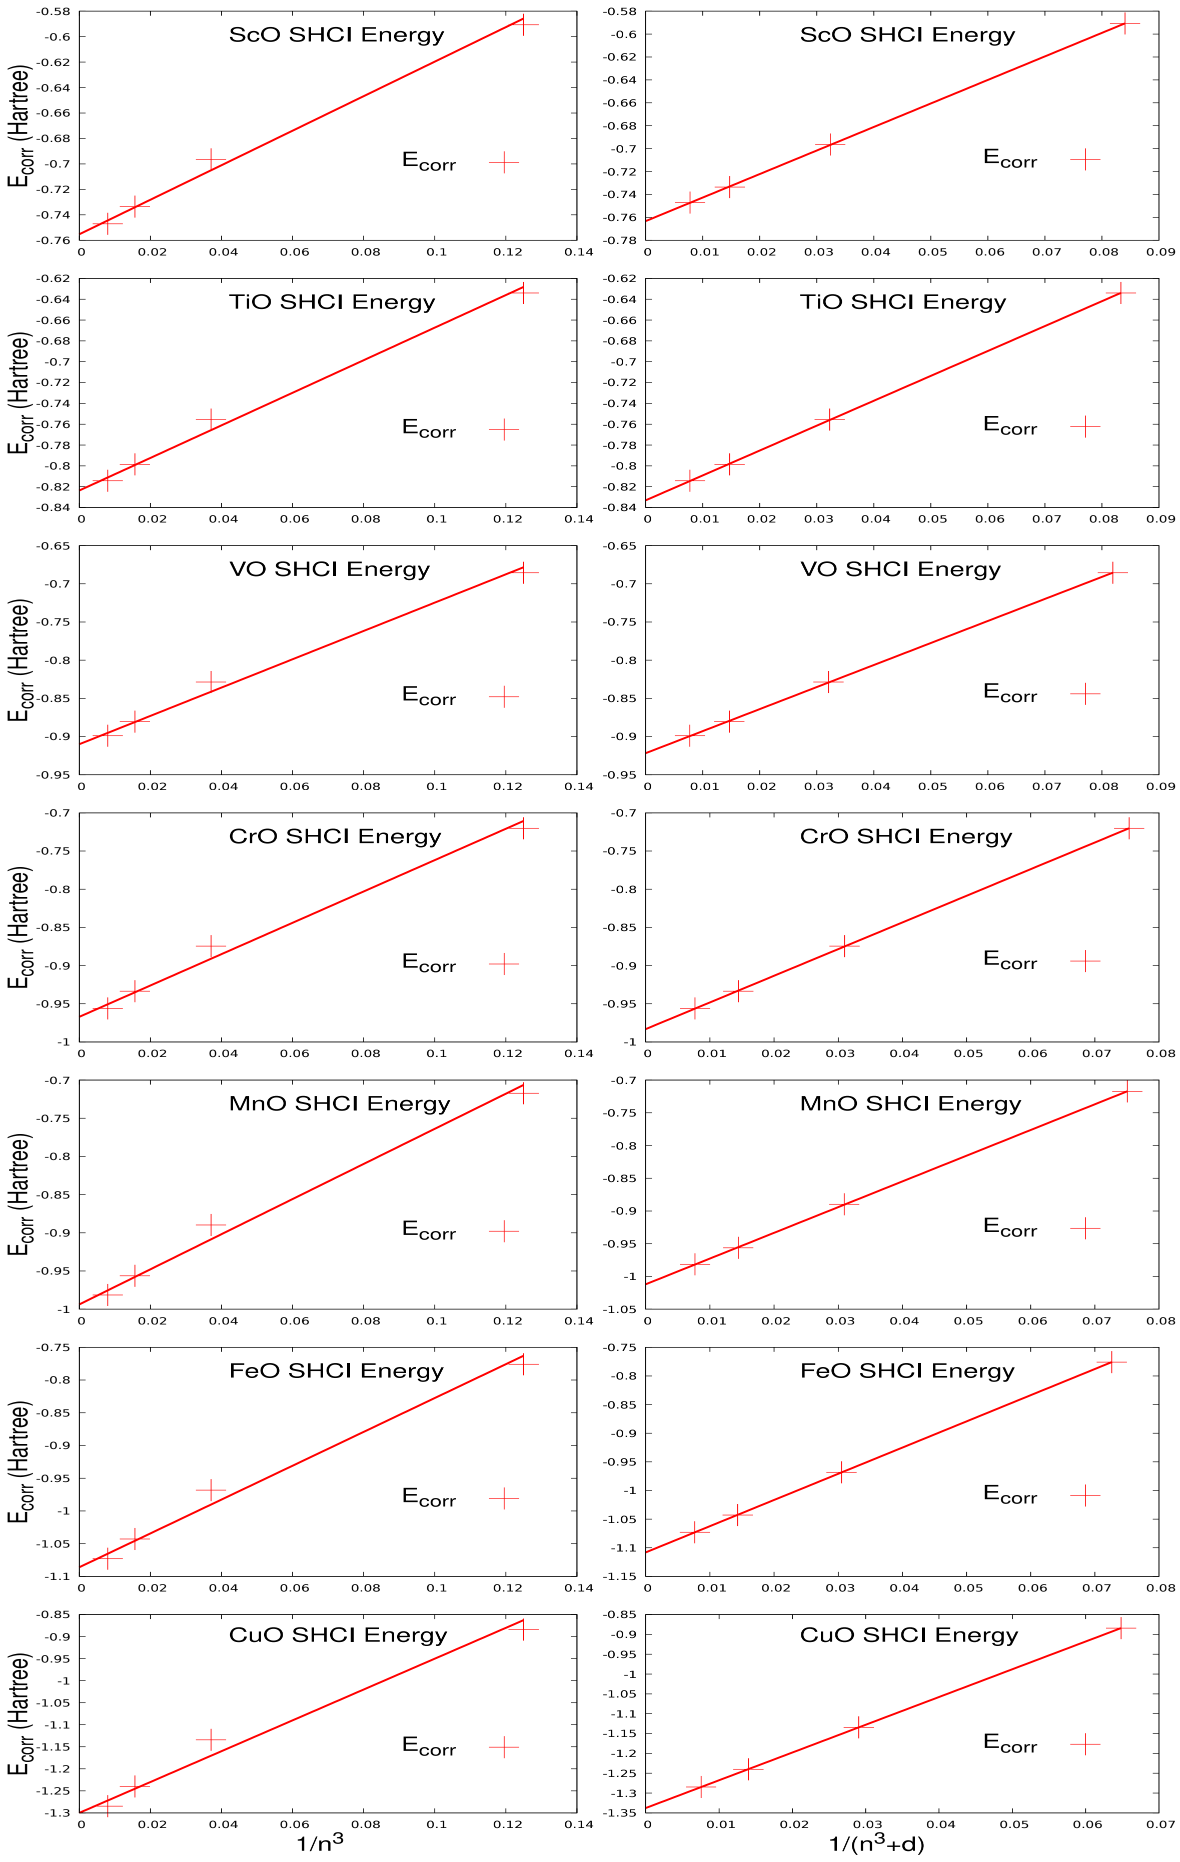


FIG. 3. Demonstration that $c/(n^3 + d)$ gives much better extrapolation fit than $c/n^3$ for transition metal oxides.

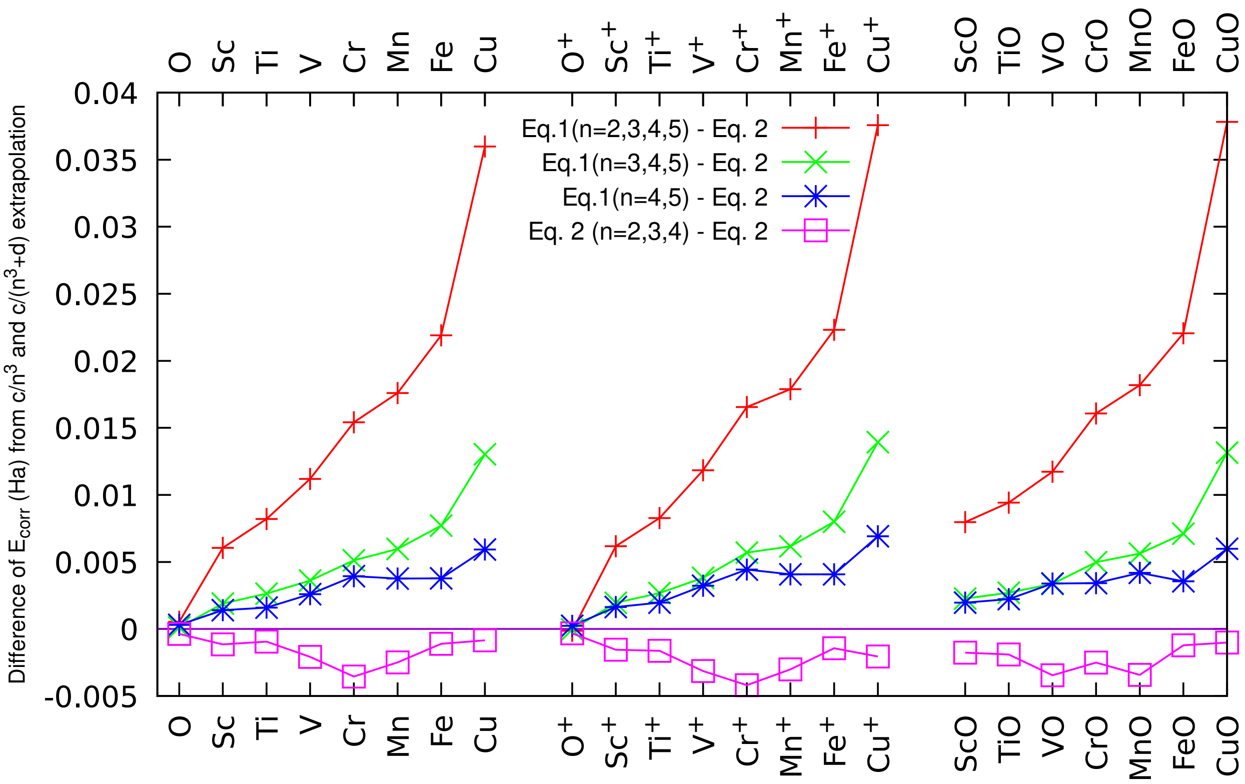


FIG. 4. Differences between the extrapolated energies using Eq. (2) with $n = 2, 3, 4, 5$ and the extrapolated energies using Eq. (1) with $n = 2, 3, 4, 5$, $n = 3, 4, 5$, and $n = 4, 5$. Also shown is the effect of using just $n = 2, 3, 4$ for the extrapolation using Eq. (1).

## II. BASIS-SET EXTRAPOLATION OF SHCI+PBE-OT TOTAL ENERGIES

In the main text, we extrapolated the SHCI+PBE-OT total energies to the CBS limit with an exponential function using $n = 3, 4, 5$:

$$E^{\text{CBS}}_{\text{SHCI+PBE-OT}} = E^{n\text{Z}}_{\text{SHCI+PBE-OT}} - a\exp\left(-bn\right), \tag{3}$$

and used them as the reference values. Some justification of this exponential form comes from the analysis of basis convergence in range-separated DFT [4].

However, we find that in situations where 5Z energies are not available, it is better to extrapolate the total energies with a modified exponential form:

$$E^{\text{CBS}}_{\text{SHCI+PBE-OT}} = E^{n\text{Z}}_{\text{SHCI+PBE-OT}} - a\exp\left(-bn^2\right). \tag{4}$$

In Table I we compare the extrapolated values from Eq. (3) using both $n = 3, 4, 5$ and $n = 2, 3, 4$, as well as those from Eq. (4) using only $n = 2, 3, 4$. For the total energies, the CBS234 scheme with Eq. (3) always gives lower estimates than the CBS345 scheme. The mean absolute deviations (MADs) between these for the total, ionization, and dissociation energies are 2.69, 0.47, and 0.98 mHa, respectively. In comparison, the CBS234 scheme with Eq. (4) gives much closer agreement with reference values: the MADs from reference values are 0.84, 0.36, and 0.60 mHa, respectively. Hence if 5Z energies are not available, it is better to extrapolate using Eq. (4) than Eq. (3). Alternatively, if only energy differences are of interest, one may as well use the QZ energies which

TABLE I. Total, ionization (for the atoms) and dissociation energies (for the monoxide molecules) obtained from extrapolating SHCI+PBE-OT energies to the CBS limit, using both $n = 2, 3, 4$ and $n = 3, 4, 5$. Unless indicated otherwise, the extrapolation uses Eq. (3). Units: Ha.

| | Total energy | | | Ionization/Dissociation energy | | |
|---|---|---|---|---|---|---|
| System | CBS234 | CBS234 Eq. (4) | CBS345 | CBS234 | CBS234 Eq. (4) | CBS345 |
| O | -15.8480 | -15.8476 | -15.8478 | 0.5004 | 0.5006 | 0.5004 |
| Sc | -46.4957 | -46.4944 | -46.4939 | 0.2411 | 0.2411 | 0.2411 |
| Ti | -58.0110 | -58.0089 | -58.0088 | 0.2506 | 0.2506 | 0.2510 |
| V | -71.2407 | -71.2379 | -71.2381 | 0.2469 | 0.2470 | 0.2475 |
| Cr | -86.8125 | -86.8079 | -86.8080 | 0.2481 | 0.2484 | 0.2489 |
| Mn | -104.1655 | -104.1609 | -104.1617 | 0.2733 | 0.2731 | 0.2730 |
| Fe | -123.7773 | -123.7730 | -123.7745 | 0.2907 | 0.2904 | 0.2903 |
| Cu | -197.6348 | -197.6305 | -197.6328 | 0.2827 | 0.2827 | 0.2839 |
| $O^+$ | -15.3476 | -15.3471 | -15.3475 | – | – | – |
| $Sc^+$ | -46.2546 | -46.2533 | -46.2528 | – | – | – |
| $Ti^+$ | -57.7604 | -57.7583 | -57.7578 | – | – | – |
| $V^+$ | -70.9938 | -70.9908 | -70.9907 | – | – | – |
| $Cr^+$ | -86.5643 | -86.5595 | -86.5591 | – | – | – |
| $Mn^+$ | -103.8921 | -103.8878 | -103.8887 | – | – | – |
| $Fe^+$ | -123.4867 | -123.4826 | -123.4843 | – | – | – |
| $Cu^+$ | -197.3520 | -197.3478 | -197.3489 | – | – | – |
| ScO | -62.6023 | -62.6004 | -62.6002 | 0.2586 | 0.2583 | 0.2585 |
| TiO | -74.1152 | -74.1128 | -74.1128 | 0.2562 | 0.2562 | 0.2562 |
| VO | -87.3361 | -87.3327 | -87.3318 | 0.2474 | 0.2472 | 0.2458 |
| CrO | -102.8349 | -102.8304 | -102.8316 | 0.1743 | 0.1749 | 0.1758 |
| MnO | -120.1588 | -120.1543 | -120.1550 | 0.1454 | 0.1458 | 0.1455 |
| FeO | -139.7821 | -139.7786 | -139.7814 | 0.1567 | 0.1580 | 0.1591 |
| CuO | -213.5938 | -213.5883 | -213.5903 | 0.1110 | 0.1101 | 0.1097 |

produce MADs of 2.87, 0.30, and 0.43 mHa for the total, ionization, and dissociation energies as shown in the main text.

## III. QUANTUM MONTE CARLO RESULTS

Real-space diffusion Monte Carlo (DMC) (see, e.g., Ref. 5) operates directly in the CBS limit. Hence it provides a potential means of testing our extrapolations to the CBS limit. However, in practice DMC requires the fixed-node approximation in order to overcome the sign problem that plagues all QMC methods. Further, when nonlocal pseudopotentials are used, DMC is forced to localize, or partially localize the pseudopotential using the so-called locality or T-moves methods, resulting in a pseudopotential localization error. Both errors depend on the trial wave function and in particular on the basis set used to construct the trial wave function. However, for typical trial wave functions, the basis-set error in DMC is typically much smaller than in other wave-function methods and these DMC errors and the variational error in variational Monte Carlo (VMC) vanish in the exact wave-function limit. Hence, by plotting the DMC energy, $E_{\mathrm{DMC}}$, versus the difference between the VMC and DMC energies, $E_{\mathrm{VMC}} - E_{\mathrm{DMC}}$, computed for a set of systematically improving wave functions and extrapolating to zero energy difference it is possible to extract the CBS energy.

A commonly used form of the trial wave function is a linear combination of configuration state

functions (CSFs) multiplied by a Jastrow factor. In our calculations we optimize three different kinds of wave-function parameters, viz., the Jastrow parameters, the CSF coefficients, and the orbital parameters, using the linear method [6–8]. The Jastrow factor has electron-nuclear, electron-electron, and electron-electron-nuclear terms of the form described in Ref. 9 (appropriately modified for a 3-dimensional system). In order to corroborate our choice of the CBS limit in the main text we performed DMC calculations for various numbers of CSFs, selected based on their coefficients in SHCI wave functions, for each of the four basis sets used in the SHCI calculations, keeping the form of the Jastrow factor fixed.

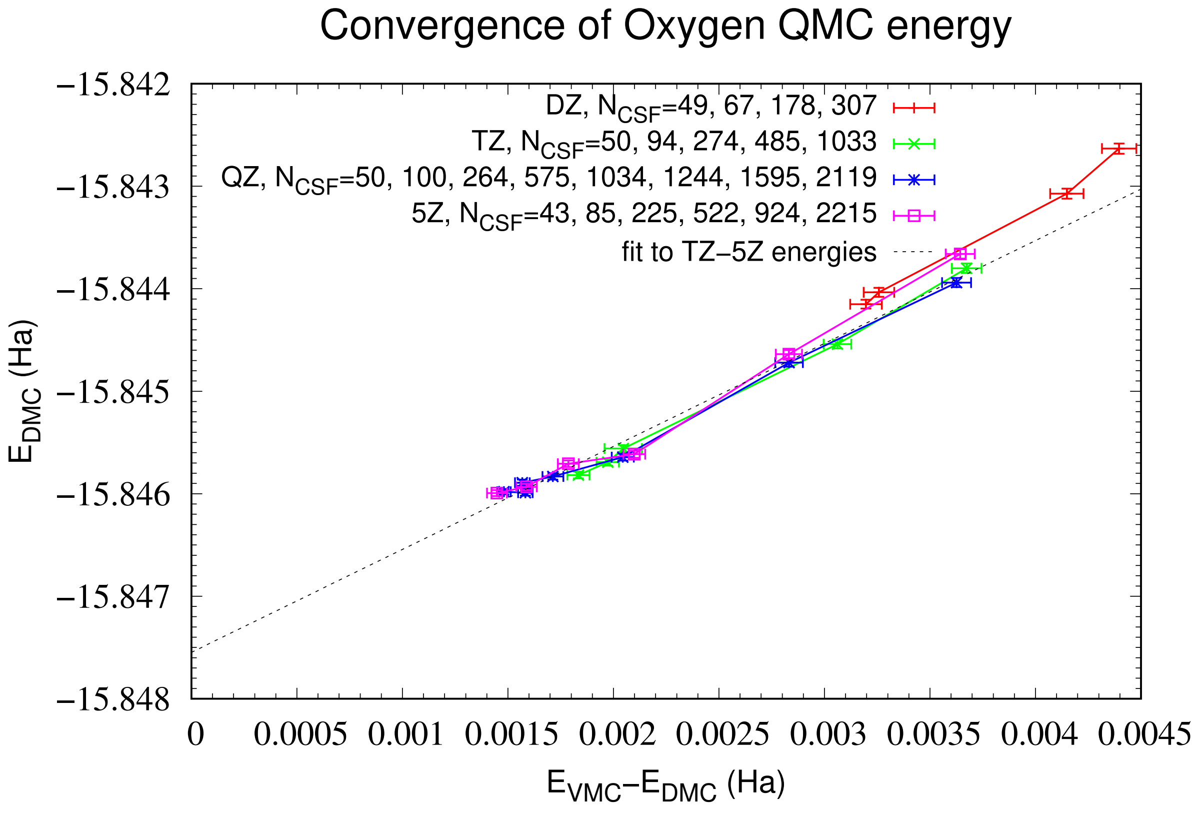


FIG. 5. Extrapolation of the DMC energy of the oxygen atom. The DMC energies versus the difference of the VMC and DMC energies using TZ-5Z basis sets lie nearly on a straight line enabling extrapolation to the zero fixed-node error limit. The number of CSFs in the wave functions is indicated in the legend.

Figure 5 shows the DMC energy versus the difference of the VMC and DMC energies. The energies from the TZ, QZ, and 5Z basis sets fall on the same curve, which is nearly a straight line whereas the energies from the DZ basis deviate from that curve a little bit. Hence, we perform a linear extrapolation of the TZ, QZ, and 5Z energies to get an estimate, -15.8475 Ha, for the CBS energy. Comparing to Table I in the main text we see that this DMC energy is very close to the SHCI+PBE-OT value of -15.8478 Ha, and to the SHCI-only value of -15.8477 Ha, but differs significantly from the SHCI+PBE-UEG value of -15.8490 Ha.

[1] T. Helgaker, W. Klopper, H. Koch, and J. Noga, J. Chem. Phys. **106**, 9639 (1997).

[2] A. Halkier, T. Helgaker, P. Jørgensen, W. Klopper, H. Koch, J. Olsen, and A. K. Wilson, Chem. Phys. Lett. **286**, 243 (1998).
[3] A. Halkier, T. Helgaker, P. Jørgensen, W. Klopper, and J. Olsen, Chem. Phys. Lett. **302**, 437 (1999).
[4] O. Franck, B. Mussard, E. Luppi, and J. Toulouse, J. Chem. Phys. **142**, 074107 (2015).
[5] J. Toulouse, R. Assaraf, and C. J. Umrigar, in *Electron Correlation in Molecules - ab initio Beyond Gaussian Quantum Chemistry*, Advances in Quantum Chemistry Vol. 73, edited by P. E. Hoggan and T. Ozdogan (Academic Press, 2016) pp. 285–314.
[6] J. Toulouse and C. J. Umrigar, J. Chem. Phys. **126**, 084102 (2007).
[7] C. J. Umrigar, J. Toulouse, C. Filippi, S. Sorella, and R. G. Hennig, Phys. Rev. Lett. **98**, 110201 (2007).
[8] J. Toulouse and C. J. Umrigar, J. Chem. Phys. **128**, 174101 (2008).
[9] A. D. Güclu, G. S. Jeon, C. J. Umrigar, and J. K. Jain, Phys. Rev. B **72**, 205327 (2005), see Eqs. 3 and 5.
